# Supplementary material for: Comparative density functional theory study for predicting oxygen reduction activity of single-atom catalyst
Source: arXiv:2209.08226 source file (2022-09-17)
Supplement: Supplementary file 1 [file Supplemental_Material.pdf]

# Supplemental Material: Comparative density functional theory study for predicting oxygen reduction activity on single-atom catalyst

Azim Fitri Zainul Abidin[1] and Ikutaro Hamada[1,*]

[1] *Department of Precision Engineering, Graduate School of Engineering, Osaka University, 2-1 Yamadaoka, Suita, Osaka 565-0871, Japan*

[*] ihamada@prec.eng.osaka-u.ac.jp

## SI. ADSORPTION GEOMETRY OF ORR INTERMEDIATES

Adsorption geometries of the ORR intermediates were optimized using different functionals, and the geometric parameters for Fe-$N_4$-C and Co-$N_4$-C are summarized in Tables SI and SII, respectively.

TABLE SI. Geometric parameters for the ORR intermediates on the Fe-$N_4$-C site. The optimized bond length between Fe and O of adsorbates ($d_{\mathrm{Fe-O}}$) and that between O atoms in adsorbate ($d_{\mathrm{O-O}}$). The unit of length is Å.

| Adsorbate | PBE | | PBE+D3 | | RPBE | | RPBE+D3 | | BEEF-vdW | |
|---|---|---|---|---|---|---|---|---|---|---|
| | $d_{\mathrm{Fe-O}}$ | $d_{\mathrm{O-O}}$ | $d_{\mathrm{Fe-O}}$ | $d_{\mathrm{O-O}}$ | $d_{\mathrm{Fe-O}}$ | $d_{\mathrm{O-O}}$ | $d_{\mathrm{Fe-O}}$ | $d_{\mathrm{O-O}}$ | $d_{\mathrm{Fe-O}}$ | $d_{\mathrm{O-O}}$ |
| $^*O_2$ | 1.749 | 1.292 | 1770 | 1.292 | 1.811 | 1.297 | 1.799 | 1.298 | 1.823 | 1.296 |
| $^*OOH$ | 1.774 | 1.483 | 1.774 | 1.485 | 1.788 | 1.502 | 1.780 | 1.500 | 1.786 | 1.502 |
| $^*O$ | 1.653 | - | 1.653 | - | 1.662 | - | 1.661 | - | 1.663 | - |
| $^*OH$ | 1.815 | - | 1.813 | - | 1.833 | - | 1.824 | - | 1.834 | - |

TABLE SII. Geometric parameters for the ORR intermediates on the Co-$N_4$-C site. The optimized bond length between Co and O of adsorbates ($d_{\mathrm{Co-O}}$), and that between O atoms in adsorbate ($d_{\mathrm{O-O}}$). The unit of length is Å.

| Adsorbate | PBE | | PBE+D3 | | RPBE | | RPBE+D3 | | BEEF-vdW | |
|---|---|---|---|---|---|---|---|---|---|---|
| | $d_{\mathrm{Co-O}}$ | $d_{\mathrm{O-O}}$ | $d_{\mathrm{Co-O}}$ | $d_{\mathrm{O-O}}$ | $d_{\mathrm{Co-O}}$ | $d_{\mathrm{O-O}}$ | $d_{\mathrm{Co-O}}$ | $d_{\mathrm{O-O}}$ | $d_{\mathrm{Co-O}}$ | $d_{\mathrm{O-O}}$ |
| $^*O_2$ | 1.885 | 1.286 | 1.883 | 1.286 | 1.913 | 1.290 | 1.934 | 1.290 | 1.914 | 1.287 |
| $^*OOH$ | 1.885 | 1.434 | 1.882 | 1.4339 | 1.911 | 1.443 | 1.925 | 1.441 | 1.909 | 1.442 |
| $^*O$ | 1.712 | - | 1.712 | - | 1.669 | - | 1.664 | - | 1.730 | - |
| $^*OH$ | 1.874 | - | 1.872 | - | 1.893 | - | 1.906 | - | 1.892 | - |

## SII. COMPARISON OF THE ADSORPTION ENERGIES FOR THE ORR INTERMEDIATES WITH PREVIOUS WORKS

TABLE SIII. Adsorption energies for the ORR adsorbates on the Fe-$N_4$-C and Co-$N_4$-C active sites obtained with PBE, along with values from the Kattel *et al.* previous works. Both active site structures used in the references were modeled from 4 × 4 graphene orthorhombic supercells. The unit of energy is eV.

| Intermediate species | Fe-$N_4$-C | Co-$N_4$-C | Fe-$N_4$-C[a] | Co-$N_4$-C[b] |
|---|---|---|---|---|
| $^*O_2$ | −1.012 | −0.736 | −0.970 | −0.670 |
| $^*$OOH | −1.801 | −1.262 | −1.720 | −1.020 |
| $^*$O | −4.482 | −3.156 | −4.530 | −3.180 |
| $^*$OH | −2.942 | −2.404 | −2.800 | −2.440 |

[a] Ref. 1
[b] Ref. 2

## SIII. CONVERGENCE STUDY

We investigate the convergence of the adsorption energies for all the ORR intermediates with respect to the kinetic energy cutoffs and **k**-point grid. In this convergence study, we only employed Fe-$N_4$-C active site with RPBE+D3, which serves as a representative functional to describe the adsorption energy.

TABLE SIV. Adsorption energies for the $^*O_2$ on the Fe-$N_4$-C obtained using difference cutoff energy and **k**-point mesh. The unit of energy is eV.

| Cutoff energy (Ry) | | **k**-point mesh | | | |
|---|---|---|---|---|---|
| $E_{cut}^{wf}$ | $E_{cut}^{den}$ | 1×1×1 | 2×2×1 | 3×3×1 | 4×4×1 |
| 50 | 500 | −0.819 | −0.834 | −0.808 | - |
| 60 | 600 | −0.819 | −0.835 | −0.808 | - |
| 70 | 700 | −0.819 | −0.835 | −0.807 | - |
| 80 | 800 | - | - | - | −0.813 |

TABLE SV. Adsorption energies for the *OOH on the Fe-$N_4$-C obtained using difference cutoff energy and **k**-point mesh. The unit of energy is eV.

| Cutoff energy (Ry) | | **k**-point mesh | | | |
|---|---|---|---|---|---|
| $E_{cut}^{wf}$ | $E_{cut}^{den}$ | 1×1×1 | 2×2×1 | 3×3×1 | 4×4×1 |
| 50 | 500 | −1.651 | −1.671 | −1.635 | - |
| 60 | 600 | −1.653 | −1.673 | −1.637 | - |
| 70 | 700 | −1.653 | −1.673 | −1.637 | - |
| 80 | 800 | - | - | - | −1.645 |

TABLE SVI. Adsorption energies for the *O on the Fe-$N_4$-C obtained using difference cutoff energy and **k**-point mesh. The unit of energy is eV.

| Cutoff energy (Ry) | | **k**-point mesh | | | |
|---|---|---|---|---|---|
| $E_{cut}^{wf}$ | $E_{cut}^{den}$ | 1×1×1 | 2×2×1 | 3×3×1 | 4×4×1 |
| 50 | 500 | −4.168 | −4.231 | −4.197 | - |
| 60 | 600 | −4.170 | −4.232 | −4.198 | - |
| 70 | 700 | −4.169 | −4.232 | −4.198 | - |
| 80 | 800 | - | - | - | −4.205 |

TABLE SVII. Adsorption energies for the *OH on the Fe-$N_4$-C obtained using difference cutoff energy and **k**-point mesh. The unit of energy is eV.

| Cutoff energy (Ry) | | **k**-point mesh | | | |
|---|---|---|---|---|---|
| $E_{cut}^{wf}$ | $E_{cut}^{den}$ | 1×1×1 | 2×2×1 | 3×3×1 | 4×4×1 |
| 50 | 500 | −2.772 | −2.773 | −2.734 | - |
| 60 | 600 | −2.774 | −2.774 | −2.736 | - |
| 70 | 700 | −2.773 | −2.774 | −2.735 | - |
| 80 | 800 | - | - | - | −2.767 |

## SIV. LATTICE CONSTANT AND ADSORPTION ENERGY WITH RPBE PAW POTENTIAL

The lattice constant and the adsorption energies for all the ORR intermediates were calculated using RPBE and RPBE+D3 functionals with RPBE PAW potentials for comparison. We confirmed that with PBE and RPBE potentials, the optimized lattice constants and the adsorption energies estimated by RPBE and RPBE+D3 functionals are almost the same.

TABLE SVIII. Optimized lattice constants for pristine graphene obtained using the RPBE and RPBE+D3 functionals with the RPBE PAW potential.

| Functional | Lattice constant (Å) |
|---|---|
| RPBE | 2.477 |
| RPBE+D3 | 2.479 |

TABLE SIX. Adsorption energies for the ORR intermediates on the Fe-$N_4$-C and Co-$N_4$-C active sites using the RPBE and RPBE+D3 functionals with the RPBE PAW potential. The unit of energy is eV.

| Intermediate species | RPBE | RPBE+D3 |
|---|---|---|
| | Fe-$N_4$-C | |
| $^*O_2$ | −0.67 | −0.81 |
| $^*$OOH | −1.48 | −1.64 |
| $^*$O | −4.13 | −4.20 |
| $^*$OH | −2.62 | −2.74 |
| | Co-$N_4$-C | |
| $^*O_2$ | −0.56 | −0.77 |
| $^*$OOH | −1.08 | −1.33 |
| $^*$O | −3.07 | −3.20 |
| $^*$OH | −2.23 | −2.43 |

## SV. FREE-ENERGY DIAGRAMS OF TM-$N_4$-C CATALYSTS AT THE PREDICTED LIMITING POTENTIAL BY BEEF-VDW FUNCTIONAL

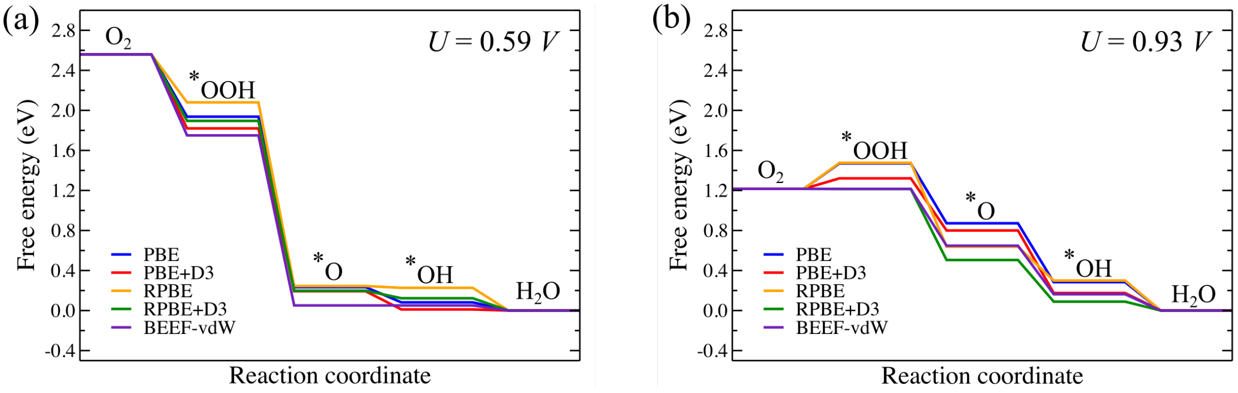


FIG. S1. Calculated free energy diagrams of ORR along the associative mechanism on (a) Fe-$N_4$-C and (b) Co-$N_4$-C catalysts. $U$ is applied electrode potential correspond to the limiting potential predicted by BEEF-vdW functional on both Fe-$N_4$-C ($U = 0.59\ V$) and Co-$N_4$-C ($U = 0.9\ V$).

## SVI. ADSORPTION ENERGIES OF THE ORR INTERMEDIATES WITH THE EFFECT OF OH-TERMINATION

TABLE SX. Adsorption energies for the ORR intermediates on the Fe(OH)-$N_4$-C and Co(OH)-$N_4$-C active sites with different functionals. The unit of energy is eV.

| Intermediate species | PBE | PBE+D3 | RPBE+D3 |
|---|---|---|---|
| | Fe-$N_4$-C | | |
| $^*O_2$ | −0.38 | −0.54 | −0.55 |
| $^*$OOH | −1.39 | −1.56 | −1.40 |
| $^*$O | −3.72 | −3.82 | −3.62 |
| $^*$OH | −2.62 | −2.76 | −2.61 |
| | Co-$N_4$-C | | |
| $^*O_2$ | −0.55 | −0.71 | −0.57 |
| $^*$OOH | −1.29 | −1.46 | −1.30 |
| $^*$O | −3.07 | −3.17 | −2.97 |
| $^*$OH | −2.49 | −2.63 | −2.48 |

## SVII. ADSORPTION FREE ENERGIES INCLUDING $O_2$ ADSORPTION PROCESS

### A. Reaction mechanism of ORR

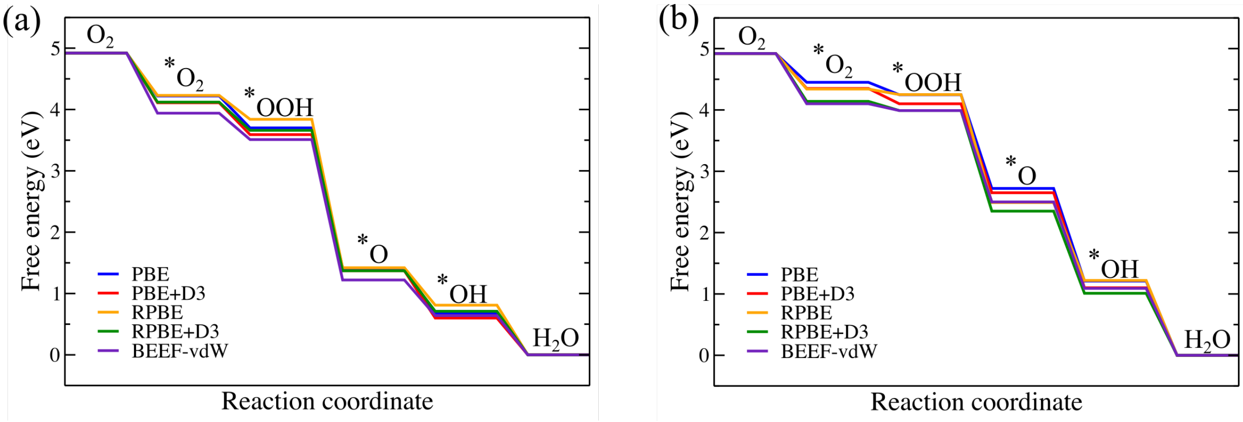


FIG. S2. Calculated free energy diagrams of ORR along the associative mechanism on (a) Fe-$N_4$-C and (b) Co-$N_4$-C catalysts at ($U = 0\ V$).

TABLE SXI. Calculated adsorption free energies for $^*O_2$, $^*OOH$, $^*O$ and $^*OH$ on Fe-$N_4$-C and Co-$N_4$-C active sites with different functionals considered. The unit of energy is eV.

| | PBE | PBE+D3 | RPBE | RPBE+D3 | BEEF-vdW |
|---|---|---|---|---|---|
| | | | Fe-$N_4$-C | | |
| $\Delta G_{^*O_2}$ | −0.67 | −0.81 | −0.69 | −0.79 | − 0.98 |
| $\Delta G_{^*OOH}$ | 3.70 | 3.59 | 3.85 | 3.66 | 3.52 |
| $\Delta G_{^*O}$ | 1.41 | 1.37 | 1.42 | 1.37 | 1.23 |
| $\Delta G_{^*OH}$ | 0.67 | 0.60 | 0.81 | 0.71 | 0.64 |
| | | | Co-$N_4$-C | | |
| $\Delta G_{^*O_2}$ | − 0.47 | −0.56 | − 0.57 | − 0.80 | − 0.81 |
| $\Delta G_{^*OOH}$ | 4.25 | 4.09 | 4.25 | 3.99 | 3.99 |
| $\Delta G_{^*O}$ | 2.72 | 2.62 | 2.49 | 2.35 | 2.50 |
| $\Delta G_{^*OH}$ | 1.21 | 1.10 | 1.22 | 1.01 | 1.09 |

## B. Reaction mechanism of ORR with OH-termination including the $O_2$ adsorption process

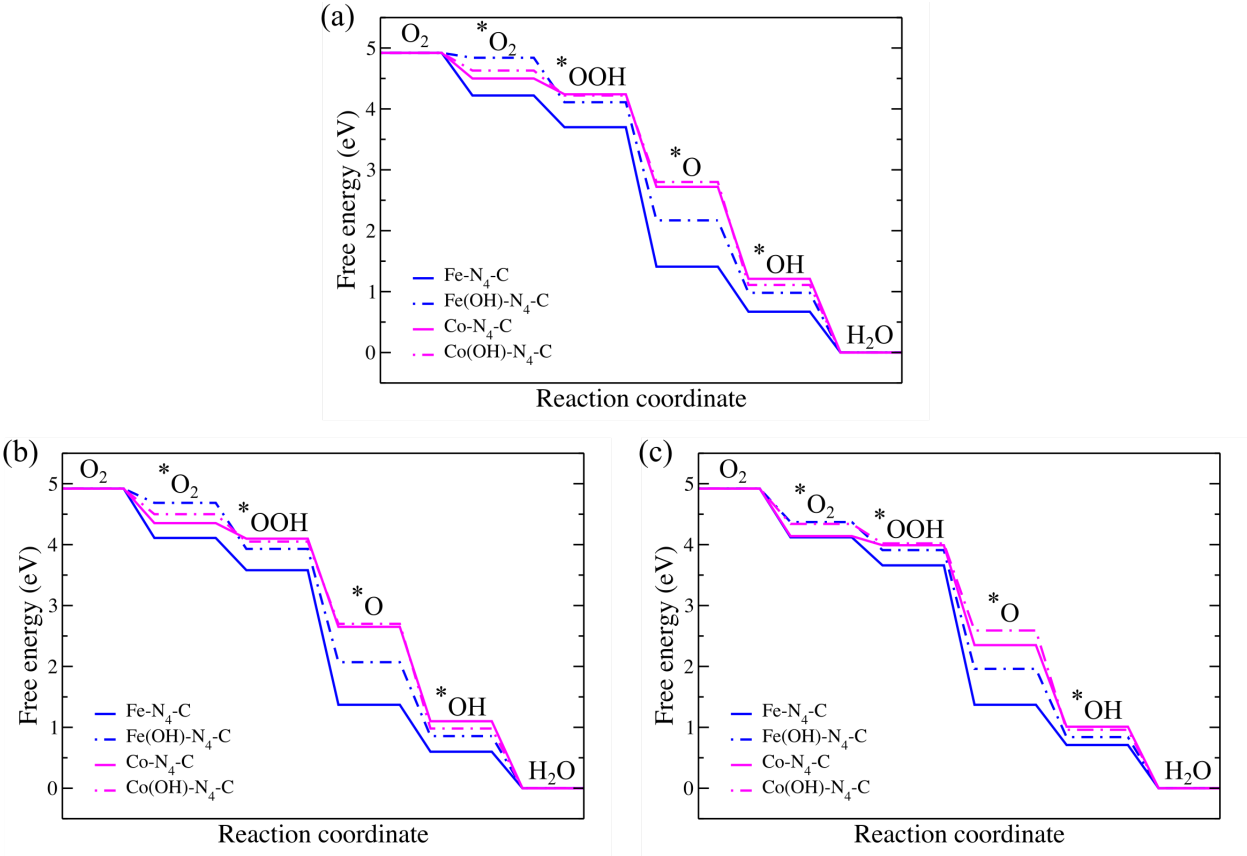


FIG. S3. Free energy diagrams of ORR along associative pathway on the Fe-$N_4$-C and Co-$N_4$-C active sites with and without OH-termination obtained using (a) PBE, (b) PBE+D3, and (c) RPBE+D3 functionals.

TABLE SXII. Calculated adsorption free energies (eV) for $^*O_2$, $^*OOH$, $^*O$ and $^*OH$ on Fe-$N_4$-C and Co-$N_4$-C active sites with PBE, PBE+D3, and RPBE+D3 functionals. The unit of energy is eV.

| | Fe-$N_4$-C | Fe(OH)-$N_4$-C | Co-$N_4$-C | Co(OH)-$N_4$-C |
|---|---|---|---|---|
| | | PBE | | |
| $\Delta G_{^*O_2}$ | −0.69 | −0.07 | −0.47 | −0.29 |
| $\Delta G_{^*OOH}$ | 3.70 | 4.11 | 4.25 | 4.22 |
| $\Delta G_{^*O}$ | 1.41 | 2.17 | 2.72 | 2.80 |
| $\Delta G_{^*OH}$ | 0.67 | 0.99 | 1.21 | 1.11 |
| | | PBE+D3 | | |
| $\Delta G_{^*O_2}$ | −0.81 | −0.23 | −0.56 | −0.41 |
| $\Delta G_{^*OOH}$ | 3.59 | 3.94 | 4.10 | 4.05 |
| $\Delta G_{^*O}$ | 1.37 | 2.07 | 2.65 | 2.70 |
| $\Delta G_{^*OH}$ | 0.60 | 0.85 | 1.10 | 0.98 |
| | | RPBE+D3 | | |
| $\Delta G_{^*O_2}$ | −0.79 | −0.54 | −0.78 | −0.57 |
| $\Delta G_{^*OOH}$ | 3.66 | 3.91 | 3.99 | 4.03 |
| $\Delta G_{^*O}$ | 1.37 | 1.96 | 2.35 | 2.59 |
| $\Delta G_{^*OH}$ | 0.71 | 0.84 | 1.01 | 0.96 |

## SVIII. ELECTRONIC STRUCTURES OF TM-$N_4$-C WITH OH-TERMINATION

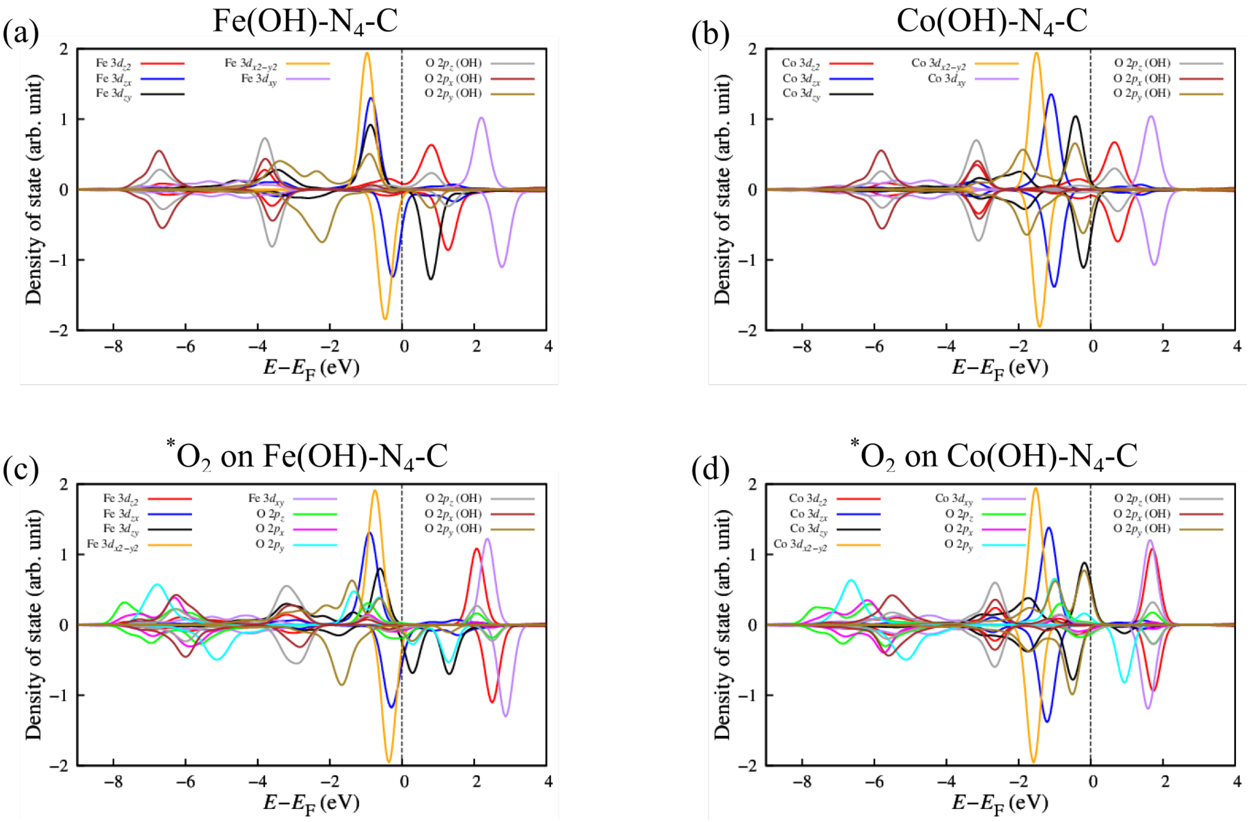


FIG. S4. The partial density of state for Fe 3$d$, Co 3$d$, and O 2$p$ of Fe(OH)-$N_4$-C and Co(OH)-$N_4$-C active sites (a), (b) without and (c), (d) with $^*O_2$ adsorbate. The origin of the energy is set to the Fermi level ($E_F$). The positive densities of states are for the spin up channel, while negative, the spin down ones.

## SIX. EFFECT OF THE HUBBARD $U$ PARAMETER ON THE TM-$N_4$-C ACTIVITY

TABLE SXIII. Adsorption energies for the ORR intermediates on the Fe-$N_4$-C and Co-$N_4$-C active sites obtained using RPBE+D3 with Hubbard $U$ ($U$ = 2 eV), along with those using RPBE+D3 ($U$ = 0 eV) . The unit of energy is eV.

| Intermediate species | $U$ = 0 eV | $U$ = 2 eV |
|---|---|---|
| | Fe-$N_4$-C | |
| $^*O_2$ | −0.81 | −0.07 |
| *OOH | −1.64 | −1.16 |
| *O | −4.20 | −3.30 |
| *OH | −2.75 | −2.42 |
| | Co-$N_4$-C | |
| $^*O_2$ | −0.77 | −0.35 |
| *OOH | −1.33 | −1.01 |
| *O | −3.20 | −2.92 |
| *OH | −2.43 | −2.12 |

TABLE SXIV. Calculated adsorption free energies (eV) for $^*O_2$, $^*OOH$, $^*O$ and $^*OH$ on Fe-$N_4$-C and Co-$N_4$-C active sites obtained using RPBE+D3 with Hubbard $U$ ($U = 2$ eV), along with those using RPBE+D3 ($U = 0$ eV). The theoretical limiting potential ($U_L$) and overpotential ($\eta_{ORR}$) is also included for further comparison. The potential determining steps (PDS) for Fe-$N_4$-C is OH formation and O formation with $U = 0$ and $U = 2$, respectively. For the Co-$N_4$-C, the PDS is OOH formation and O formation with $U = 0$ and $U = 2$, respectively. The unit of energy is eV and potential is volt.

| | $U = 0$ eV | $U = 2$ eV |
|---|---|---|
| | Fe-$N_4$-C | |
| $\Delta G_{^*O_2}$ | $-0.79$ | $-0.05$ |
| $\Delta G_{^*OOH}$ | 3.66 | 4.14 |
| $\Delta G_{^*O}$ | 1.37 | 2.27 |
| $\Delta G_{^*OH}$ | 0.71 | 1.03 |
| $U_L$ | 0.66 | 0.77 |
| $\eta_{ORR}$ | 0.56 | 0.46 |
| | Co-$N_4$-C | |
| $\Delta G_{^*O_2}$ | $-0.78$ | $-0.35$ |
| $\Delta G_{^*OOH}$ | 3.99 | 4.31 |
| $\Delta G_{^*O}$ | 2.35 | 2.64 |
| $\Delta G_{^*OH}$ | 1.01 | 1.32 |
| $U_L$ | 0.93 | 0.60 |
| $\eta_{ORR}$ | 0.30 | 0.60 |

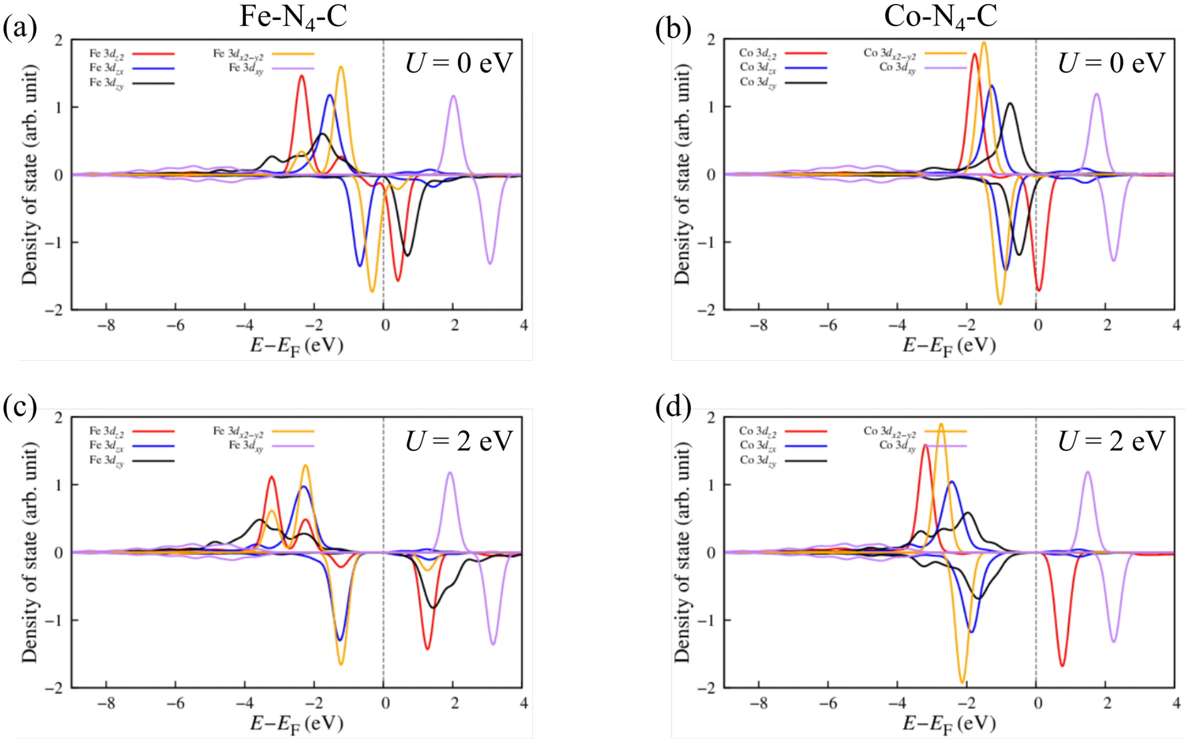


FIG. S5. The partial density of state for Fe 3$d$, and Co 3$d$ of Fe-$N_4$-C and Co-$N_4$-C active sites with different $U$ values, (a) and (b) for $U$ = 0 eV, (c) and (d) for $U$ = 2 eV. The origin of the energy is set to the Fermi level ($E_F$). The positive densities of states are for the spin up channel, while negative, the spin down ones.

## SX. FREE ENERGY CONTRIBUTIONS

TABLE SXV. Calculated zero point energy ($E_{ZPE}$) corrections of the systems obtained with different functionals. The unit of energy is eV.

| Intermediate species | PBE | PBE+D3 | RPBE | RPBE+D3 | BEEF-vdW |
|---|---|---|---|---|---|
| | | | Isolated molecule | | |
| $H_2$ | 0.273 | 0.273 | 0.273 | 0.273 | 0.273 |
| $H_2O$ | 0.570 | 0.570 | 0.570 | 0.570 | 0.570 |
| | | | Fe-$N_4$-C | | |
| $^*O_2$ | 0.148 | 0.142 | 0.139 | 0.141 | 0.142 |
| $^*$OOH | 0.425 | 0.426 | 0.420 | 0.421 | 0.421 |
| $^*$O | 0.069 | 0.069 | 0.068 | 0.068 | 0.068 |
| $^*$OH | 0.347 | 0.347 | 0.345 | 0.348 | 0.349 |
| | | | Co-$N_4$-C | | |
| $^*O_2$ | 0.135 | 0.141 | 0.136 | 0.138 | 0.137 |
| $^*$OOH | 0.438 | 0.439 | 0.438 | 0.439 | 0.439 |
| $^*$O | 0.059 | 0.059 | 0.061 | 0.061 | 0.061 |
| $^*$OH | 0.330 | 0.033 | 0.329 | 0.327 | 0.328 |

TABLE SXVI. Calculated entropy contribution to the Free energy ($TS$) of the systems at $T$ = 298.15 $K$, obtained with different functionals. The unit of energy is eV.

| Intermediate species | PBE | PBE+D3 | RPBE | RPBE+D3 | BEEF-vdW |
|---|---|---|---|---|---|
| | | | Isolated molecule | | |
| $H_2$ | 0.400 | 0.400 | 0.400 | 0.400 | 0.400 |
| $H_2O$ | 0.670 | 0.670 | 0.670 | 0.670 | 0.670 |
| | | | $Fe$-$N_4$-$C$ | | |
| $^*O_2$ | 0.147 | 0.151 | 0.157 | 0.152 | 0.153 |
| $^*$OOH | 0.188 | 0.187 | 0.192 | 0.192 | 0.192 |
| $^*$O | 0.067 | 0.066 | 0.066 | 0.066 | 0.066 |
| $^*$OH | 0.101 | 0.100 | 0.102 | 0.100 | 0.101 |
| | | | $Co$-$N_4$-$C$ | | |
| $^*O_2$ | 0.170 | 0.162 | 0.172 | 0.168 | 0.170 |
| $^*$OOH | 0.194 | 0.191 | 0.193 | 0.193 | 0.191 |
| $^*$O | 0.071 | 0.071 | 0.076 | 0.077 | 0.077 |
| $^*$OH | 0.083 | 0.083 | 0.083 | 0.087 | 0.087 |

[1] S. Kattel, P. Atanassov, and B. Kiefer, A density functional theory study of oxygen reduction reaction on non-PGM Fe–$N_x$–C electrocatalysts, Physical Chemistry Chemical Physics **16**, 13800 (2014).

[2] S. Kattel, P. Atanassov, and B. Kiefer, Catalytic activity of Co–$N_x$/C electrocatalysts for oxygen reduction reaction: a density functional theory study, Physical Chemistry Chemical Physics **15**, 148 (2013).
